# Supplementary material for: ClioQuery: Interactive Query-Oriented Text Analytics for Comprehensive Investigation of Historical News Archives
Source: arXiv:2204.04694 source file (2022-04-10)
Supplement: Supplementary file 2 [file Supplemental_Expert_Interview_Script.pdf]

# Script: Expert Interview Study

## Pretask and Objectives [10 minutes]

Hi ___. Thanks again for agreeing to participate in this study. I am working with a group trying to understand how to design software for social researchers analyzing news documents. During this interview, you will try out our software and then answer a few questions about your experiences.

In preparing for this session you mentioned an interest in how the *New York Times* editorial board discussed *X* during the late 1980s to the late 2000s. In all of the experiments today, we will be using a collection of *New York Times* editorials published between 1987-2007 which include the word X.

*New York Times* editorials appear in the opinion section, do not have authors and express the beliefs of the paper's editorial staff.

Can you tell me a little bit more about why you are interested in what the *New York Times* editorial board says about *X*?

**Follow up 1:** Solicit details about the participant's interest in *X* based on their own work and field.

**Follow up 2**: To encourage time-based questions, ask about what events were happening during this time span and how the *NYT* editorial board might have responded to and influenced such events.

## Tutorial [7 minutes]

Now I'm going to take a few minutes to talk you through ClioQuery. Feel free to interrupt me with any questions [I will resume the script once answered]. Can you open the URL posted to Zoom chat?

For this tutorial we will be using a corpus of *New York Times* editorials which contain the word "drugs" published between 1987 and 2007.

At the top of the ClioQuery interface is a black time series graph. See how the time series graph goes from 1987 to 2007? The height of the line in the graph shows how many editorials were

published each year during that time period. If you hover over 1994 in the chart you can see there were about 27 editorials published in 1994 which mention drugs.

Now if you look below the graph, you can see that there is a feed showing all of those editorials in chronological order. Each item in the feed shows the headline and publication date of an editorial.

**Queries, document feed and document viewer**

Now try searching for some word related to your topic by filling out "Query Search" at the top of the interface. ClioQuery will go find all editorials mentioning drugs that contain your query term. [pause]

You can see that the plot updates to show how often your query word occurs in each year of the corpus, using a purple line.

You might have noticed that the Document Feed now shows only those documents which mention your query.

Now, in the feed, try clicking "Show [4] more" beneath the [third] result. That will show you all of the query mentions in the document. You can also click "collapse" to hide these query mentions.

Try clicking one of the query mentions. It will open up the document in the Document Viewer to the right. Do you see how you can see the mention in context in the Document Viewer? If you hover over the mention you can see that it becomes dark yellow in both the feed and the document viewer.

**Subqueries**

If you look to the top right screen you will see a box that says "filter by subquery". This helps you find search results that contain a query term, much like using control F in a web browser.

[Suggest a subquery and search].

Now that you have searched for [subquery] do you see how all of the squares in the Document Feed are now white or green. Darker green squares mean the article contains many mentions of your subquery; white squares mean that the article does not contain your subquery. The darker the green, the more times the document mentions your subquery.

Now try scrolling down through the feed. [Look for example]. See how there is a short sentence that starts with your query term and ends with the filter term? Wherever possible, our system will try to make snippets that have this format, describing a relationship between your query and your subquery. Now go ahead and unset your subquery by clicking the little x.

**Filtering**

Ok now we are back to our main query. Do you see how there is a purple square beside each publication date in the Document Feed? That purple square shows how many times a document mentions your query term. Darker shades of purple mean that the document has more mentions.

If you look at the slider where is says "Filter by # mentions," you can see a legend showing the exact number of mentions in each document. Try moving that slider to the right to the number 3. Notice that the feed adjusts to show only documents containing at least 3 mentions of your query term.

You can also use the date pickers at the top of the interface to narrow down to certain dates

**History tracking**

ClioQuery includes bookmarking and history tracking features so you can keep track of what you have read.

Try clicking the star beside one of the headlines. Notice that on the right hand side of the interface, the number of bookmarked documents now shows 1.

If you look very closely at the little lines below the time series plot you will notice that one of them has turned dark red. Those lines are called rug points. There should be 1 red rug point. That is the story you just bookmarked.

Now try clicking some other story. The story opens in the document viewer. Do you see how the count of read documents increased by 1 on the right hand side? If you look closely, you will also see that one of the black rug points has also turned light grey.

Try clicking a few more stories. See how the number of read stories goes up? There are more grey rug points on the plot.

**Wrap up**

That covers the major features of our system. You will also notice some smaller things as you start using the tool. But I think that is everything to explain before you get started.

**Note**: Get informal feedback: do they ask questions, do they understand system, do they pick up the UI quickly, do they seem to like it?

# Main Task [30 minutes]

**Think aloud instructions**: At the start of this interview, we discussed a research question related to *X.* [Remind them of question.] Now I'd like you to research that question using our system. As you use our software, please talk through what you are trying to do. For instance, you might say "I am clicking this headline because I want to read the whole story." Be sure to say if you get stuck or frustrated, or if the system does things that are unexpected. Can you go ahead and share your screen?

**Observe**: what actions do they take and why?

**Follow ups:**

For any action, give them a chance to do it and then ask:

- Why did you do that?
- Do you like or dislike this feature in the system and why?

# Post Task [13 minutes]

For this portion, screenshare shows the *researcher's* screen.

**Q1, word-for-word script.** When you want to investigate a query in a corpus (like in this study) what tools do you use? For instance, do you use Proquest or microfilm?

Follow up 1: what do you like or dislike about those tools?

Follow up 2: what are the advantages and disadvantages of our proposed software system, as compared to tools you normally use.

**Q2, word-for-word script.** Earlier, we discussed your interest in X and formed a research question about X. Did our system help you answer your research question?

Follow up: repeat answer and ask *what* about the system was helpful or unhelpful?

**Q3, word-for-word script.** Our system displayed all mentions of your query term in a single, chronological Document Feed. Was this feature helpful or unhelpful?

Follow up: can you talk about *why* you like/dislike/don't care about this feature

**Q4, word-for-word script.** Our system displayed shortened sentences highlighted in-context in the Document Viewer. Were these yellow highlighted text fragments helpful or unhelpful?

Follow up: can you talk about *why* you like/dislike/don't care about this feature

**Q5, word-for-word script.** Our system showed yellow highlighted text in two places, the Document Feed and Document Viewer. Did you find one feature more useful than the other?

Follow up: can you talk about *why* you like/dislike/don't care about this feature

**Q6, word-for-word script.** Our system includes a graph showing the number of query mentions through time. Did you find this useful?

Follow up: can you talk about *why* you like/dislike/don't care about this feature

**Q7, word-for-word script.** Our system included features to help you filter and keep track of query results (e.g. counts of read documents)**.** Did you find these features helpful or unhelpful?

Follow up: can you talk about *why* you like/dislike/don't care about this feature

**Q8, word-for-word script.** When you use a traditional search engine like Google it shows you a ranked list of documents**.** Our system uses filters to help you select sets of documents, instead of showing a ranked list. Do you think ranked lists or filters are better for historical research?

Follow up: can you talk about *why* you like/dislike/don't care about this feature
