# Supplementary material for: ClioQuery: Interactive Query-Oriented Text Analytics for Comprehensive Investigation of Historical News Archives
Source: arXiv:2204.04694 source file (2022-04-10)
Supplement: Supplementary file 3 [file Supplemental_Needfinding_Interview_Script.pdf]

## Background

1. Can you tell me about a time when you searched successfully in a digital archive for news articles or other timestamped media sources?
2. What tools do you use when searching digital archives, especially for news periodicals?
3. What do you like about those tools?
4. What do you dislike about those tools?

## Keyword search and time

5. Say there is more in a digital news archive than you could possibly read. What methods do you use to choose what to examine?

    e.g. Search engines? Read microfilm? Narrow by time? Follow citations? Topic model?

    Pick one follow up: Do you ever use search engines? When you start a search, do you usually understand exactly what you are looking for? How do you decide what to search for? When using search engines, do you ever limit results to a specific time period (if so why?).

6. Many news documents are written on specific days (e.g. January 15th, 1988). But historians often study a range of dates (e.g. the late 1980s or post World War II). How do you keep track of what happened when?

    e.g. Do you make timelines? Take notes? Keep track in your head?

    If they use a system ask about it.

    If they keep track mentally, ask then to talk through an example of a time they kept track of events.

## Contextual information

7. What metadata helps you decide if you should open an article during a news search?

    e.g. publication, date, a section like opinion/sports

## Comprehensiveness

8. When you are searching an archive, how do you know that it is OK to stop looking?

9. When would it be OK for a historical researcher not to read all possible evidence?

## Transparency, control, and trustworthiness

10. When you are making a claim about primary news sources, how do you ensure that other historians will trust your conclusions?
    a. E.g. take photos of source and publish along with work, detailed quotation, citation, reference to other work in the area

## Feedback on the prototype

**100% open-ended**

What features of the software design do you like?
What features of the software design do you dislike?
How would you imagine using this system?
Can you give an example of how you might use this software for a prior project?
What features might you want?
