# Supplementary material for: ClioQuery: Interactive Query-Oriented Text Analytics for Comprehensive Investigation of Historical News Archives
Source: arXiv:2204.04694 source file (2022-04-10)
Supplement: Supplementary file 4 [file codebook.tex]

\documentclass[acmsmall,screen,review,anonymous]{acmart}

\newcount\Comments  % 0 suppresses notes to selves in text
\Comments=1   % TODO: set to 0 for final version

% for comments
\usepackage{color}

\definecolor{CCPurple}{rgb}{.405, .144, .450} % hex 672573
\definecolor{darkgreen}{rgb}{.106, .471, .216}
\definecolor{gold}{RGB}{240,205,17}

\newcommand{\kibitz}[2]{\ifnum\Comments=1\textcolor{#1}{#2}\fi}

\newcommand{\ours}{\textsc{ClioQuery}}

 % min w/o word wrap

\usepackage{multirow}
\usepackage{makecell}
\usepackage{subcaption}
\usepackage{bm}
\usepackage{enumitem}
\usepackage[normalem]{ulem} 

%%
%% \BibTeX command to typeset BibTeX logo in the docs
\AtBeginDocument{%
  \providecommand\BibTeX{{%
    \normalfont B\kern-0.5em{\scshape i\kern-0.25em b}\kern-0.8em\TeX}}}

%% Rights management information.  This information is sent to you
%% when you complete the rights form.  These commands have SAMPLE
%% values in them; it is your responsibility as an author to replace
%% the commands and values with those provided to you when you
%% complete the rights form.
\setcopyright{acmcopyright}
\copyrightyear{2021}
\acmYear{2021}
\acmDOI{xxx}

%%
%% These commands are for a JOURNAL article.
\acmJournal{TIIS}
\acmVolume{xx}
\acmNumber{xx}
\acmArticle{ACM Article No}
\acmMonth{1}

\begin{document}

%%
%% If your work has an appendix, this is the place to put it.

\section*{Codebook for expert interview study}

\subsection*{Historical sensemaking}
The quote explains, articulates, or offers backstory about a hypothesis regarding specific historical events or processes. The user finds evidence for or against their historical hypothesis, or discovers new evidence that casts a prior historical hypothesis in a different light. The user explores and analyzes historical information based on knowledge of the domain.

\subsection*{\ours~Features}
The quote addresses some specific feature of the \ours~system including the Document Feed, Document Viewer, Time Series Plot, rug points, filtering system, history tracking system, color coding, in-text highlighting and text simplification. This theme also encompasses suggested features for future versions of \ours~(e.g. complex Boolean queries or wildcards).

\subsection*{Comprehensiveness}
This quote addresses the role of comprehensive search in the historical research process. Comprehensive search refers to gathering all available evidence and reviewing all evidence to reach conclusions.

\subsection*{Context in historical research}
This quote addresses the role of context in the historical research process. Historians and archivists sometimes say that they need context to evaluate evidence. For instance, some historians may say they need to understand a quote from a news story in context. Context includes things like when a story was published, and where a story appeared in the paper.

\subsection*{Bias and transparency}
This quote addresses the role of bias and transparency in historical research. Some users sometimes stress the importance of directly and neutrally observing evidence in archives, without computers exerting any sway over their research process. 

\subsection*{Current practices}
This quote addresses the tools and methods that historians and archivists currently use to search archives. For instance, quotes describing reading historical books, visiting physical archives, using search engines, using microfilm, using microfiche, and using specific services like Google, the Internet Archive or ProQuest are all coded as current practices. 

\end{document}
